# Supplementary material for: Locating and Controlling Implicit Personalization in Large Language Models
Source: arXiv:2608.11735 source file (2026-08-12)
Supplement: Supplementary file 6 [file appendix_crossscale.tex]

\section{Cross-Scale Replication}
\label{sec:app-crossscale}

The correlation and composition experiments of \S\ref{sec:corr} and
\S\ref{sec:lin} run on all five models, but the direction ablation of
\S\ref{sec:abl} is restricted, for compute reasons, to the three
7--8B models (\S\ref{sec:models}). The remainder of this appendix
isolates the two 14B models---Qwen3-14B and Phi-4---and verifies that the
two model-general findings survive the scale increase: $\Delta W$ still
tracks the per-sample behavioral shift, and the mixed-cue direction still
decomposes into its single-cue components. Neither 14B model was run
through the ablation, so their contribution here is detection and
composition evidence, not causal removal.

\begin{table*}[t]
\centering \small
\begin{tabular}{lrccc c}
\toprule
Model & $N_L$ & $L^\star$ & $\bar\rho$ & $\bar\rho_{\times}$ & Abl. \\
\midrule
Llama-3-8B & 32 & 19--31 & .703--.712 & .145--.169 & \textbullet \\
Mistral-7B & 32 & 15--31 & .668--.680 & .116--.167 & \textbullet \\
Qwen3-8B   & 36 & 17--31 & .615--.638 & .053--.061 & \textbullet \\
Qwen3-14B  & 40 & 1--31  & .578--.581 & .043--.053 & -- \\
Phi-4      & 40 & 6--31  & .666--.680 & .122--.140 & -- \\
\bottomrule
\end{tabular}
\caption{Cross-scale summary. $N_L$: transformer depth. $L^\star$:
span of the mediating layer set used in \S\ref{sec:lin} (union of the
top-10 NIE layers over the pair's conditions; the union has $12$--$15$
distinct layers on the 7--8B models and $16$--$26$ at 14B). $\bar\rho$:
own-sample composition fit; $\bar\rho_{\times}$: cross-sample control,
each a range over the three dimension pairs. ``Abl.'' marks the models
carried into the \S\ref{sec:abl} direction ablation (\textbullet)
versus those contributing detection and composition only (--).}
\label{tab:crossscale}
\end{table*}

\paragraph{Layer sets.}
Table~\ref{tab:crossscale} gives, per model, the mediating layer set
$L^\star$ (from the intersectional analysis: the union of the top-10
NIE layers over the conditions entering each pair) alongside the
composition fit. At 14B the retained $L^\star$ is more dispersed than
at 7--8B: on Qwen3-14B it spans layers $1$--$31$ ($23$--$26$ distinct
layers per pair) and on Phi-4 layers $6$--$31$ ($16$ layers), against
the tight $15$--$31$ band of the smaller models. The union reaches
early layers at 14B, but the highest-NIE layer in every condition is
still late (layers $28$--$31$), so the mid-to-late localization from
\S\ref{sec:corr} carries over.

One caveat concerns the search window. The top-10 NIE ranking
(Appendix~\ref{sec:app-patching}) was taken over a fixed window of the
first $32$ layers on every model; recovery was computed at every
layer, but the ranking that defines $L^\star$ considered only layers
$0$--$31$. For the three deeper models---Qwen3-8B ($36$ layers) and
the two 14B models ($40$ layers)---this excludes the topmost layers
($32$--$35$ and $32$--$39$), several of which carry post-attention
recovery comparable to, and in places exceeding, the retained layers.
Because those excluded layers are themselves late and the retained
$L^\star$ already concentrates mid-to-late, widening the window would
only extend the same late-layer region; it does not change the
localization or any result below. We report $L^\star$ as it was
actually used.

\paragraph{Correlation replicates (\S\ref{sec:corr}).}
On the two universal anchors, per-sample $\Delta W$ tracks behavior on
both 14B models. Against CAR, Qwen3-14B \texttt{race\_black} reaches
$r = +0.82$ and \texttt{age\_child} $r = +0.60$; Phi-4 reaches $+0.73$
and $+0.51$. Against SED-description the same four cells give
$+0.49/+0.52$ (Qwen3-14B) and $+0.62/+0.61$ (Phi-4). A significant shift
appears on $7/9$ conditions for each 14B model, and---as on the
smaller models---the per-sample $r$ collapses toward zero exactly
where the behavior does (\texttt{race\_white} on both;
\texttt{age\_adult}). The full per-condition grid, including both 14B
columns, is Table~\ref{tab:phase1}; these anchor correlations use the
per-condition top-10 layers, which lie inside the same $0$--$31$
window discussed above.

\paragraph{Linear composition replicates (\S\ref{sec:lin}).}
The mixed-cue direction decomposes substantially linearly at both
14B models. Averaged over samples and cells, the own-sample fit is
$\bar\rho \in [0.578, 0.581]$ on Qwen3-14B and $[0.666, 0.680]$ on
Phi-4 (Table~\ref{tab:crossscale}), inside the $[0.578, 0.712]$ range
that holds across all five models. The cross-sample control---which
decomposes $v_{AB}^{(i)}$ onto single-cue vectors from a
\emph{different} sample of the same cell---drops to $[0.043, 0.053]$
on Qwen3-14B and $[0.122, 0.140]$ on Phi-4, far below the own-sample
fit and near the reliability reference. The decomposition is
therefore sample-specific at 14B as well, not a generic cell-level
geometry. Qwen3-14B gives the lowest own-sample fit of the five
models and the narrowest own-vs-cross gap, consistent with its
being the weakest of the five on SED-description in
Table~\ref{tab:phase1}: the finding holds at the largest scale we
test, but least strongly there.
